# Supplementary material for: Conditional Choice Probability Estimation of Dynamic Discrete Choice Models with 2-period Finite Dependence
Source: arXiv:2405.12467 source file (2024-05-21)
Supplement: Supplementary file 1 [file appendix_sdg_convergence.tex]

\begin{figure}
  \centering
  \caption{State Space $X = 64$, $\gamma_a = 1$}
  \begin{subfigure}[b]{0.32\textwidth}
      \centering
      \includegraphics[width=\textwidth]{fig/fig_weight_2period_gammaa_1_o_2_z_2_x_64_rate_0.050_batch_1_hessian_0.png}
      \caption{$\alpha=0.05$}
  \end{subfigure}
  \hfill
  \begin{subfigure}[b]{0.32\textwidth}
      \centering
      \includegraphics[width=\textwidth]{fig/fig_weight_2period_gammaa_1_o_2_z_2_x_64_rate_0.100_batch_1_hessian_0.png}
      \caption{$\alpha=0.1$}
  \end{subfigure}
  \hfill
  \begin{subfigure}[b]{0.32\textwidth}
      \centering
      \includegraphics[width=\textwidth]{fig/fig_weight_2period_gammaa_1_o_2_z_2_x_64_rate_0.200_batch_1_hessian_0.png}
      \caption{$\alpha=0.2$}
  \end{subfigure}

    \hfill
    \begin{subfigure}[b]{0.32\textwidth}
      \centering
      \includegraphics[width=\textwidth]{fig/fig_weight_2period_gammaa_1_o_2_z_2_x_64_rate_0.300_batch_1_hessian_0.png}
      \caption{$\alpha=0.3$}
  \end{subfigure}
  \hfill
  \begin{subfigure}[b]{0.32\textwidth}
      \centering
      \includegraphics[width=\textwidth]{fig/fig_weight_2period_gammaa_1_o_2_z_2_x_64_rate_0.500_batch_1_hessian_0.png}
      \caption{$\alpha=0.5$}
  \end{subfigure}
  \hfill
  \begin{subfigure}[b]{0.32\textwidth}
      \centering
      \includegraphics[width=\textwidth]{fig/fig_weight_2period_gammaa_1_o_2_z_2_x_64_rate_0.700_batch_1_hessian_0.png}
      \caption{$\alpha=0.7$}
  \end{subfigure}
     \label{fig:graph_1}
\end{figure}

\begin{figure}
  \centering
  \caption{State Space $X = 486$, $\gamma_a = 1$}
  \begin{subfigure}[b]{0.32\textwidth}
      \centering
      \includegraphics[width=\textwidth]{fig/fig_weight_2period_gammaa_1_o_3_z_3_x_486_rate_0.050_batch_1_hessian_0.png}
      \caption{$\alpha=0.05$}
  \end{subfigure}
  \hfill
  \begin{subfigure}[b]{0.32\textwidth}
      \centering
      \includegraphics[width=\textwidth]{fig/fig_weight_2period_gammaa_1_o_3_z_3_x_486_rate_0.100_batch_1_hessian_0.png}
      \caption{$\alpha=0.1$}
  \end{subfigure}
  \hfill
  \begin{subfigure}[b]{0.32\textwidth}
      \centering
      \includegraphics[width=\textwidth]{fig/fig_weight_2period_gammaa_1_o_3_z_3_x_486_rate_0.200_batch_1_hessian_0.png}
      \caption{$\alpha=0.2$}
  \end{subfigure}

    \hfill
    \begin{subfigure}[b]{0.32\textwidth}
      \centering
      \includegraphics[width=\textwidth]{fig/fig_weight_2period_gammaa_1_o_3_z_3_x_486_rate_0.300_batch_1_hessian_0.png}
      \caption{$\alpha=0.3$}
  \end{subfigure}
  \hfill
  \begin{subfigure}[b]{0.32\textwidth}
      \centering
      \includegraphics[width=\textwidth]{fig/fig_weight_2period_gammaa_1_o_3_z_3_x_486_rate_0.500_batch_1_hessian_0.png}
      \caption{$\alpha=0.5$}
  \end{subfigure}
  \hfill
  \begin{subfigure}[b]{0.32\textwidth}
      \centering
      \includegraphics[width=\textwidth]{fig/fig_weight_2period_gammaa_1_o_3_z_3_x_486_rate_0.700_batch_1_hessian_0.png}
      \caption{$\alpha=0.7$}
  \end{subfigure}
     \label{fig:graph_2}
\end{figure}

\begin{figure}
  \centering
  \caption{State Space $X = 1024$, $\gamma_a = 1$}
  \begin{subfigure}[b]{0.32\textwidth}
      \centering
      \includegraphics[width=\textwidth]{fig/fig_weight_2period_gammaa_1_o_2_z_4_x_1024_rate_0.050_batch_1_hessian_0.png}
      \caption{$\alpha=0.05$}
  \end{subfigure}
  \hfill
  \begin{subfigure}[b]{0.32\textwidth}
      \centering
      \includegraphics[width=\textwidth]{fig/fig_weight_2period_gammaa_1_o_2_z_4_x_1024_rate_0.100_batch_1_hessian_0.png}
      \caption{$\alpha=0.1$}
  \end{subfigure}
  \hfill
  \begin{subfigure}[b]{0.32\textwidth}
      \centering
      \includegraphics[width=\textwidth]{fig/fig_weight_2period_gammaa_1_o_2_z_4_x_1024_rate_0.200_batch_1_hessian_0.png}
      \caption{$\alpha=0.2$}
  \end{subfigure}

    \hfill
    \begin{subfigure}[b]{0.32\textwidth}
      \centering
      \includegraphics[width=\textwidth]{fig/fig_weight_2period_gammaa_1_o_2_z_4_x_1024_rate_0.300_batch_1_hessian_0.png}
      \caption{$\alpha=0.3$}
  \end{subfigure}
  \hfill
  \begin{subfigure}[b]{0.32\textwidth}
      \centering
      \includegraphics[width=\textwidth]{fig/fig_weight_2period_gammaa_1_o_2_z_4_x_1024_rate_0.500_batch_1_hessian_0.png}
      \caption{$\alpha=0.5$}
  \end{subfigure}
  \hfill
  \begin{subfigure}[b]{0.32\textwidth}
      \centering
      \includegraphics[width=\textwidth]{fig/fig_weight_2period_gammaa_1_o_2_z_4_x_1024_rate_0.700_batch_1_hessian_0.png}
      \caption{$\alpha=0.7$}
  \end{subfigure}
     \label{fig:graph_3}
\end{figure}
